# Supplementary material for: Sea urchin sperm exploit extremum seeking control to find the egg
Source: arXiv:2108.13634 source file (2022-10-04)
Supplement: Supplementary file 1 [file SI.pdf]

## Supporting Information Text

If the angular velocity components  $\omega_{\perp}(\cdot)$  and  $\omega_{\parallel}(\cdot)$  are given by:

$$\omega_{\perp}(t) = \omega_{\perp,0} + \omega_{\perp,1}\eta(t), \quad [1]$$

$$\omega_{\parallel}(t) = \omega_{\parallel,0} + \omega_{\parallel,1}\eta(t), \quad [2]$$

then we may rewrite the rotational kinematics as:

$$\dot{\mathbf{R}}(t) = \mathbf{R}(t) \left( \hat{\boldsymbol{\Omega}}_0 + \hat{\boldsymbol{\Omega}}_1 \eta(t) \right) \quad [3]$$

where the vectors  $\boldsymbol{\Omega}_0$  and  $\boldsymbol{\Omega}_1$  are given by:

$$\boldsymbol{\Omega}_0 = \begin{bmatrix} \omega_{\parallel,0} \\ 0 \\ \omega_{\perp,0} \end{bmatrix}, \quad \boldsymbol{\Omega}_1 = \begin{bmatrix} \omega_{\parallel,1} \\ 0 \\ \omega_{\perp,1} \end{bmatrix} \quad [4]$$

Let  $\mathbf{R}_0(t) = \exp(\hat{\boldsymbol{\Omega}}_0 t)$  and  $\bar{\mathbf{R}}(t) = \mathbf{R}(t)\mathbf{R}_0(t)^{\top}$ , and compute:

$$\mathbf{R}_0(t) = \begin{pmatrix} \frac{\omega_{\perp,0}^2}{\omega^2} \cos(\omega t) + \frac{\omega_{\parallel,0}^2}{\omega^2} & -\frac{\omega_{\perp,0}}{\omega} \sin(\omega t) & \frac{\omega_{\perp,0}\omega_{\parallel,0}}{\omega^2} (1 - \cos(\omega t)) \\ \frac{\omega_{\perp,0}}{\omega} \sin(\omega t) & \cos(\omega t) & -\frac{\omega_{\parallel,0}}{\omega} \sin(\omega t) \\ \frac{\omega_{\perp,0}\omega_{\parallel,0}}{\omega^2} (1 - \cos(\omega t)) & \frac{\omega_{\parallel,0}}{\omega} \sin(\omega t) & \frac{\omega_{\perp,0}^2}{\omega^2} \cos(\omega t) + \frac{\omega_{\parallel,0}^2}{\omega^2} \end{pmatrix} \quad [5]$$

Then, observe that:

$$\begin{aligned} \dot{\mathbf{p}}(t) &= \mathbf{R}(t)\mathbf{V} = \mathbf{R}(t)\mathbf{R}_0(t)^{\top}\mathbf{R}_0(t)\mathbf{V} = \bar{\mathbf{R}}(t)\mathbf{R}_0(t)\mathbf{V} \\ \dot{\bar{\mathbf{R}}}(t) &= \dot{\mathbf{R}}(t)\mathbf{R}_0(t)^{\top} + \mathbf{R}(t)\dot{\mathbf{R}}_0(t)^{\top} = \mathbf{R}(t)\hat{\boldsymbol{\Omega}}_0\mathbf{R}_0(t)^{\top} + \eta(t)\mathbf{R}(t)\hat{\boldsymbol{\Omega}}_1\mathbf{R}_0(t)^{\top} - \mathbf{R}(t)\hat{\boldsymbol{\Omega}}_0\mathbf{R}_0(t)^{\top} \\ &= \mathbf{R}(t)\mathbf{R}_0(t)^{\top}\mathbf{R}_0(t)\hat{\boldsymbol{\Omega}}_1\mathbf{R}_0(t)^{\top}\eta(t) \end{aligned}$$

where  $\omega = \sqrt{\omega_{\perp,0}^2 + \omega_{\parallel,0}^2}$ . Let  $v > 0$ ,  $|\omega_{\perp,0}| > 0$ , and :

$$\mathbf{e}_1 = \begin{pmatrix} \frac{\omega_{\parallel,0}}{\omega} \\ 0 \\ \frac{\omega_{\perp,0}}{\omega} \end{pmatrix}, \quad \mathbf{e}_3(\omega t) = \begin{pmatrix} \frac{\omega_{\perp,0}}{\omega} \cos(\omega t) \\ \sin(\omega t) \\ -\frac{\omega_{\parallel,0}}{\omega} \cos(\omega t) \end{pmatrix} \quad [6]$$

then observe that  $\|\mathbf{e}_1\| = \|\mathbf{e}_3(\cdot)\| = 1$ , and that:

$$\mathbf{R}_0(t)\mathbf{V} = \frac{v\omega_{\parallel,0}}{\omega}\mathbf{e}_1 + \frac{v\omega_{\perp,0}}{\omega}\mathbf{e}_3(\omega t) \quad [7]$$

$$\mathbf{R}_0(t)\hat{\boldsymbol{\Omega}}_1\mathbf{R}_0(t)^{\top} = \left( \omega_{\perp,1}\frac{\omega_{\perp,0}}{\omega} + \omega_{\parallel,1}\frac{\omega_{\parallel,0}}{\omega} \right) \hat{\mathbf{V}}_1 + \left( \omega_{\parallel,1}\frac{\omega_{\perp,0}}{\omega} - \frac{\omega_{\parallel,0}}{\omega}\omega_{\perp,1} \right) \hat{\mathbf{V}}_3(\omega t) \quad [8]$$

Consequently, we have that:

$$\dot{\mathbf{p}}(t) = \bar{\mathbf{R}}(t) \left( \frac{v\omega_{\perp,0}}{\omega}\mathbf{e}_3(\omega t) + \frac{v\omega_{\parallel,0}}{\omega}\mathbf{e}_1 \right) \quad [9]$$

If we integrate both sides with respect to  $t$ , we obtain:

$$\mathbf{p}(\sigma)|_0^t = \frac{v\omega_{\perp,0}}{\omega} \int_0^t \bar{\mathbf{R}}(\sigma)\mathbf{e}_3(\omega\sigma) d\sigma + \frac{v\omega_{\parallel,0}}{\omega} \int_0^t \bar{\mathbf{R}}(\sigma)\mathbf{e}_1 d\sigma \quad [10]$$

Integrating the first term on the right hand side by parts yields:

$$\mathbf{p}(s)|_0^t = \frac{v\omega_{\perp,0}}{\omega^2} \bar{\mathbf{R}}(\sigma)\mathbf{e}_2(\omega\sigma)|_0^t - \frac{v\omega_{\perp,0}}{\omega^2} \int_0^t \bar{\mathbf{R}}(\sigma)\mathbf{R}_0(\sigma)\hat{\boldsymbol{\Omega}}_1\mathbf{R}_0(\sigma)^{\top}\mathbf{e}_2(\omega\sigma)\eta(\sigma) d\sigma + \frac{v\omega_{\parallel,0}}{\omega} \int_0^t \bar{\mathbf{R}}(\sigma)\mathbf{e}_1 d\sigma \quad [11]$$

where

$$\mathbf{e}_2(\omega\sigma) = \int \mathbf{e}_3(\omega\sigma) d(\omega\sigma) = \begin{pmatrix} \frac{\omega_{\perp,0}}{\omega} \sin(\omega\sigma) \\ -\cos(\omega\sigma) \\ -\frac{\omega_{\parallel,0}}{\omega} \sin(\omega\sigma) \end{pmatrix} \quad [12]$$

Observe that  $\mathbf{e}_2(\cdot)$  is periodic with zero average,  $\|\mathbf{e}_2(\cdot)\| = 1$ , and that:

$$\mathbf{e}_1 \times \mathbf{e}_2(\omega t) = \mathbf{e}_3(\omega t) \quad [13]$$

$$\mathbf{e}_2(\omega t) \times \mathbf{e}_3(\omega t) = \mathbf{e}_1 \quad [14]$$

$$\mathbf{e}_3(\omega t) \times \mathbf{e}_1 = \mathbf{e}_2(\omega t) \quad [15]$$

$$\mathbf{e}_2(\omega t + \phi_0) = \cos(\phi_0)\mathbf{e}_2(\omega t) + \sin(\phi_0)\mathbf{e}_3(\omega t) \quad [16]$$

where  $\times$  denotes the cross product between 3D vectors. Move the first term on the right hand side in Eq 11 to the left hand side and differentiate both sides again to obtain:

$$\frac{d}{dt} \left( \mathbf{p}(t) - \frac{v\omega_{\perp,0}}{\omega^2} \bar{\mathbf{R}}(t) \mathbf{e}_2(\omega t) \right) = \bar{\mathbf{R}}(t) \left( -\frac{v\omega_{\perp,0}}{\omega^2} \mathbf{R}_0(t) \hat{\boldsymbol{\Omega}}_1 \mathbf{R}_0(t)^\top \mathbf{e}_2(\omega t) \eta(t) + \frac{v\omega_{\parallel,0}}{\omega} \mathbf{e}_1 \right) \quad [17]$$

If we make the identifications:

$$\boldsymbol{\delta}(\omega t) = \frac{v\omega_{\perp,0}}{\omega} \mathbf{e}_2(\omega t) \quad [18]$$

$$\bar{\mathbf{V}} = \frac{v\omega_{\parallel,0}}{\omega} \mathbf{e}_1 \quad [19]$$

$$\bar{\mathbf{p}}(t) = \mathbf{p}(t) - \frac{1}{\omega} \bar{\mathbf{R}}(t) \boldsymbol{\delta}(\omega t) \quad [20]$$

$$\hat{\boldsymbol{\Omega}}_\eta(\omega t) = \mathbf{R}_0(t) \hat{\boldsymbol{\Omega}}_1 \mathbf{R}_0(t)^\top \quad [21]$$

$$\mathbf{V}_\eta(\omega t) = -\hat{\boldsymbol{\Omega}}_\eta(\omega t) \boldsymbol{\delta}(\omega t) \quad [22]$$

then the kinematics become:

$$\dot{\bar{\mathbf{p}}}(t) = \bar{\mathbf{R}}(t) \mathbf{V}_\eta(\omega t) \frac{\eta(t)}{\omega} + \bar{\mathbf{R}}(t) \bar{\mathbf{V}} \quad [23]$$

$$\dot{\bar{\mathbf{R}}}(t) = \bar{\mathbf{R}}(t) \hat{\boldsymbol{\Omega}}_\eta(\omega t) \eta(t) \quad [24]$$

We compute the expressions for  $\mathbf{V}_\eta, \boldsymbol{\Omega}_\eta$  which turn out to be:

$$\boldsymbol{\Omega}_\eta(\omega t) = \left( \omega_{\parallel,1} \frac{\omega_{\parallel,0}}{\omega} + \omega_{\perp,1} \frac{\omega_{\perp,0}}{\omega} \right) \mathbf{e}_1 + \left( \omega_{\perp,1} \frac{\omega_{\parallel,0}}{\omega} - \omega_{\parallel,1} \frac{\omega_{\perp,0}}{\omega} \right) \mathbf{e}_3(\omega t) \quad [25]$$

$$\mathbf{V}_\eta(\omega t) = \frac{v\omega_{\perp,0}}{\omega} \left( \omega_{\perp,1} \frac{\omega_{\parallel,0}}{\omega} - \omega_{\parallel,1} \frac{\omega_{\perp,0}}{\omega} \right) \mathbf{e}_1 - \frac{v\omega_{\perp,0}}{\omega} \left( \omega_{\parallel,1} \frac{\omega_{\parallel,0}}{\omega} + \omega_{\perp,1} \frac{\omega_{\perp,0}}{\omega} \right) \mathbf{e}_3(\omega t) \quad [26]$$

Observe that the feedback coefficients  $\mathbf{V}_\eta, \boldsymbol{\Omega}_\eta$  are periodic with non zero average in general, whereas the periodic perturbation  $\boldsymbol{\delta}(\omega t)$  always has zero average. Let  $\varepsilon = \frac{1}{\omega}$ , and observe that the instantaneous local concentration  $c(\mathbf{p}(t))$  may be approximated by its first order Taylor series:

$$c(\mathbf{p}(t)) = c(\bar{\mathbf{p}}(t) + \varepsilon \bar{\mathbf{R}}(t) \boldsymbol{\delta}(\omega t)) = c(\bar{\mathbf{p}}(t)) + \varepsilon \nabla c(\bar{\mathbf{p}}(t))^\top \bar{\mathbf{R}}(t) \boldsymbol{\delta}(\omega t) + \mathcal{O}(\varepsilon^2) \quad [27]$$

as long as  $\|\boldsymbol{\delta}(\omega t)\| \cdot \|\nabla c(\bar{\mathbf{p}}(t))\| = \mathcal{O}(1)$  and  $0 < \varepsilon \ll 1$ . By employing the fundamental theorem of calculus, the average local concentration  $c(\bar{\mathbf{p}}(t))$  can be written as:

$$c(\bar{\mathbf{p}}(t)) = c(\bar{\mathbf{p}}(t)) + \int_t^t \nabla c(\bar{\mathbf{p}}(\tau))^\top \dot{\bar{\mathbf{p}}}(\tau) d\tau = c(\bar{\mathbf{p}}(t)) + \int_t^t \nabla c(\bar{\mathbf{p}}(\tau))^\top \bar{\mathbf{R}}(\tau) (\varepsilon \mathbf{V}_\eta(\omega \tau) \eta(\tau) + \bar{\mathbf{V}}) d\tau \quad [28]$$

Hence, the instantaneous local concentration can be expressed as:

$$c(\mathbf{p}(t)) = c(\bar{\mathbf{p}}(t)) + \int_t^t \nabla c(\bar{\mathbf{p}}(\tau))^\top \bar{\mathbf{R}}(\tau) \bar{\mathbf{V}} d\tau + \varepsilon \nabla c(\bar{\mathbf{p}}(t))^\top \bar{\mathbf{R}}(t) \boldsymbol{\delta}(\omega t) + \varepsilon \int_t^t \nabla c(\bar{\mathbf{p}}(\tau))^\top \bar{\mathbf{R}}(\tau) \mathbf{V}_\eta(\omega \tau) \eta(\tau) d\tau + \mathcal{O}(\varepsilon^2) \quad [29]$$

In the absence of feedback (i.e. when  $\eta(t) = 0$ ), the instantaneous local concentration is given by:

$$c(\mathbf{p}(t)) = c(\bar{\mathbf{p}}(t)) + \int_t^t \nabla c(\bar{\mathbf{p}}(\tau))^\top \bar{\mathbf{R}}(\tau) \bar{\mathbf{V}} d\tau + \varepsilon \nabla c(\bar{\mathbf{p}}(t))^\top \bar{\mathbf{R}}(t) \boldsymbol{\delta}(\omega t) + \mathcal{O}(\varepsilon^2) \quad [30]$$

Over a short time duration  $t \leq t' \leq t + \varepsilon$ , the integral in the expression for  $c(\mathbf{p}(t))$  may be approximated by its first order Taylor series:

$$\int_t^{t'} \nabla c(\bar{\mathbf{p}}(\tau))^\top \bar{\mathbf{R}}(\tau) \bar{\mathbf{V}} d\tau \approx \nabla c(\bar{\mathbf{p}}(t))^\top \bar{\mathbf{R}}(t) \bar{\mathbf{V}} (t' - t) + \mathcal{O}(\varepsilon^2) \approx \varepsilon \nabla c(\bar{\mathbf{p}}(t))^\top \bar{\mathbf{R}}(t) \bar{\mathbf{V}} \omega \Delta t + \mathcal{O}(\varepsilon^2) \quad [31]$$

where  $\Delta t = t' - t$ . The same applies to the average position  $\bar{\mathbf{p}}(t) \approx \bar{\mathbf{p}}(t) + \mathcal{O}(\varepsilon)$  and average orientation  $\bar{\mathbf{R}}(t) \approx \bar{\mathbf{R}}(t) + \mathcal{O}(\varepsilon)$ . Hence, over an  $\mathcal{O}(\varepsilon)$  time duration  $t \leq t' \leq t + \varepsilon$ , the instantaneous local concentration  $c(\mathbf{p}(t))$  can be approximated by:

$$c(\mathbf{p}(t)) = c(\bar{\mathbf{p}}(t)) + \varepsilon \nabla c(\bar{\mathbf{p}}(t))^\top \bar{\mathbf{R}}(t) (\bar{\mathbf{V}} \omega \Delta t + \boldsymbol{\delta}(\omega t)) + \mathcal{O}(\varepsilon^2) \quad [32]$$

A time scale change to  $\sigma = \omega \Delta t$  puts the instantaneous local concentration in the form:

$$c(\mathbf{p}(\sigma)) = c(\bar{\mathbf{p}}(t)) + \varepsilon \nabla c(\bar{\mathbf{p}}(t))^\top \bar{\mathbf{R}}(t) (\bar{\mathbf{V}} \sigma + \boldsymbol{\delta}(\sigma)) + \mathcal{O}(\varepsilon^2) \quad [33]$$

The stimulus to which the signaling pathway is exposed due to the binding of the SAP molecules may be taken as:

$$s(t) \approx c(\mathbf{p}(t)) \quad [34]$$

Hence, the approximate form of the stimulus in the time scale  $\sigma$  starting at  $t$  is:

$$s(\sigma) \approx c(\bar{\mathbf{p}}(t)) + \varepsilon \|\nabla c(\bar{\mathbf{p}}(t))\| \left( \frac{\nabla c(\bar{\mathbf{p}}(t))^\top}{\|\nabla c(\bar{\mathbf{p}}(t))\|} \bar{\mathbf{R}}(t) \bar{\mathbf{V}} \sigma + \frac{\nabla c(\bar{\mathbf{p}}(t))^\top}{\|\nabla c(\bar{\mathbf{p}}(t))\|} \bar{\mathbf{R}}(t) \boldsymbol{\delta}(\sigma) \right) + \mathcal{O}(\varepsilon^2) \quad [35]$$

Recalling that the triad  $\mathbf{e}_1, \mathbf{e}_2(\omega t), \mathbf{e}_3(\omega t)$  forms an orthonormal basis, and that  $\mathbf{e}_2(\omega t)$  completes a full rotation in the plane that is orthogonal to  $\mathbf{e}_1$  with frequency  $\omega$ , one can see that:

$$\frac{\nabla c(\bar{\mathbf{p}}(t))^\top}{\|\nabla c(\bar{\mathbf{p}}(t))\|} \bar{\mathbf{R}}(t) \mathbf{e}_1 = \cos(\theta(t)) \quad [36]$$

$$\frac{\nabla c(\bar{\mathbf{p}}(t))^\top}{\|\nabla c(\bar{\mathbf{p}}(t))\|} \bar{\mathbf{R}}(t) \mathbf{e}_2(\sigma) = \sqrt{1 - \cos(\theta(t))^2} \sin(\sigma + \phi_0(t)) \quad [37]$$

where  $\theta(t)$  is the angle between the normalized gradient  $\bar{\mathbf{R}}(t)^\top \frac{\nabla c(\bar{\mathbf{p}}(t))}{\|\nabla c(\bar{\mathbf{p}}(t))\|}$  and the vector  $\mathbf{e}_1$ , and the angle  $\phi_0(t)$  depends on the initial angle between  $\mathbf{e}_2(\sigma)$  and the projection of  $\bar{\mathbf{R}}(t)^\top \frac{\nabla c(\bar{\mathbf{p}}(t))}{\|\nabla c(\bar{\mathbf{p}}(t))\|}$  on the plane that is orthogonal to  $\mathbf{e}_1$ . Consequently, the stimulus maybe approximated by:

$$s(\sigma) \approx c(\bar{\mathbf{p}}(t)) + \varepsilon v \|\nabla c(\bar{\mathbf{p}}(t))\| \left( \frac{\omega_{\parallel,0}}{\omega} \cos(\theta(t)) \sigma + \frac{\omega_{\perp,0}}{\omega} \sqrt{1 - \cos(\theta(t))^2} \sin(\sigma + \phi_0(t)) \right) + \mathcal{O}(\varepsilon^2) \quad [38]$$

This form of the input passes through the model of the signaling pathway given in the time scale  $\sigma$  by:

$$\sigma_1 \omega \frac{d\zeta_1}{d\sigma} = \zeta_2(\sigma) - \zeta_1(\sigma) \quad [39]$$

$$\sigma_2 \omega \frac{d\zeta_2}{d\sigma} = s(\sigma) - \zeta_2(\sigma) \quad [40]$$

$$\zeta(\sigma) = \zeta_2(\sigma) - \zeta_1(\sigma) \quad [41]$$

$$\mu \omega \frac{d\rho}{d\sigma} = \rho(\sigma) (1 - (\rho(\sigma) \zeta(\sigma))^2) \quad [42]$$

$$\eta(\sigma) = \rho(\sigma) \zeta(\sigma) \quad [43]$$

The first three equations [39]-[41] are decoupled from the fourth. Moreover, they are linear with a transfer function  $G(\lambda)$  given by:

$$G(\lambda) = \mathcal{L} \left\{ \frac{\zeta(t)}{s(t)} \right\} = \frac{\sigma_1 \omega \lambda}{(1 + \sigma_1 \omega \lambda)(1 + \sigma_2 \omega \lambda)} \quad [44]$$

For simplicity, we assume that  $\sigma_1 = \sigma_2 = \sigma_c = \mathcal{O}(\varepsilon)$  so that  $\sigma_c \omega = \mathcal{O}(1)$  and the transients vanish fast enough without affecting the quasi steady behavior. A direct application of linear analysis techniques yields the following expression for the quasi-steady signal  $\zeta(t)$  under the stimulus input given by [38]:

$$\zeta(\sigma) \approx \varepsilon v \sigma_c \omega \|\nabla c(\bar{\mathbf{p}}(t))\| \left( \frac{\omega_{\parallel,0}}{\omega} \cos(\theta(t)) + \frac{v \omega_{\perp,0}}{\omega} \frac{1}{(1 + \omega^2 \sigma_c^2)} \sqrt{1 - \cos(\theta(t))^2} \sin(\sigma + \phi + \phi_0) \right) \quad [45]$$

where  $\phi$  is the phase contribution of the transfer function  $G(\lambda)$ , and is such that:

$$\tan(\phi) = \frac{1 - \sigma_c^2 \omega^2}{2 \omega \sigma_c} \quad [46]$$

Next, this quasi steady  $\zeta(\sigma)$  is applied as an input to the adaptation equation [42]. We observe that  $\zeta$  has the form:

$$\zeta(\sigma) = \nu_0 (\nu_1 + \nu_2 \sin(\omega t + \phi + \phi_0)) \quad [47]$$

where the constants  $\nu_1, \nu_2$  are given by:

$$\nu_0 = \varepsilon v \sigma_c \omega \|\nabla c(\bar{\mathbf{p}}(t))\| > 0, \quad \nu_1 = \frac{\omega_{\parallel,0}}{\omega} \cos(\theta(t)), \quad \nu_2 = \frac{\omega_{\perp,0}}{\omega} \frac{1}{(1 + \omega^2 \sigma_c^2)} \sqrt{1 - \cos(\theta(t))^2} \quad [48]$$

Hence, a quasi steady approximation of equation [42] becomes:

$$\mu\omega \frac{d\rho}{d\sigma} = \rho(\sigma) \left(1 - \nu_0^2 \rho(\sigma)^2 (\nu_1 + \nu_2 \sin(\sigma + \phi + \phi_0))^2\right) \quad [49]$$

This is a first order nonlinear differential equation with periodic coefficients. Fortunately, an exact solution may be obtained and the quasi steady state approximation of the solution is given by the expression:

$$\rho(\sigma) = \frac{1}{\nu_0 \sqrt{\nu_1^2 + \frac{\nu_2^2}{2} - \frac{4\nu_1\nu_2(\mu\omega \cos(\sigma+\phi+\phi_0)-2\sin(\sigma+\phi+\phi_0))}{\mu^2\omega^2+4} - \frac{\nu_2^2(\mu\omega \sin(2(\sigma+\phi+\phi_0))+\cos(2(\sigma+\phi+\phi_0)))}{2\mu^2\omega^2+2}} \quad [50]$$

Consequently, the quasi steady signal  $\eta(\sigma)$  is given by:

$$\eta(\sigma) = \frac{\nu_1 + \nu_2 \sin(\sigma + \phi + \phi_0)}{\sqrt{\nu_1^2 + \frac{\nu_2^2}{2} - \frac{4\nu_1\nu_2(\mu\omega \cos(\sigma+\phi+\phi_0)-2\sin(\sigma+\phi+\phi_0))}{\mu^2\omega^2+4} - \frac{\nu_2^2(\mu\omega \sin(2(\sigma+\phi+\phi_0))+\cos(2(\sigma+\phi+\phi_0)))}{2\mu^2\omega^2+2}}} \quad [51]$$

We observe that the signal  $\eta(\sigma)$  is independent of  $\nu_0$  (i.e. the magnitude of the gradient). If we make a time variable change to  $\tau = \sigma + \phi + \phi_0$  and expand  $\eta(t)$  as a Fourier series in  $\tau$ , we obtain:

$$\eta(\tau) \approx \beta_1(\nu_1, \nu_2) + \beta_2(\nu_1, \nu_2) \sin(\tau) + \beta_3(\nu_1, \nu_2) \cos(\tau) + \text{H.O.H} \quad [52]$$

where the coefficients  $\beta_1, \beta_2, \beta_3$  are given by the integrals:

$$\beta_1(\nu_1, \nu_2) = \frac{1}{2\pi} \int_{-\pi}^{\pi} \frac{(\nu_1 + \nu_2 \sin(\tau))}{\sqrt{\nu_1^2 + \frac{\nu_2^2}{2} - \frac{4\nu_1\nu_2(\mu\omega \cos(\tau)-2\sin(\tau))}{\mu^2\omega^2+4} - \frac{\nu_2^2(\mu\omega \sin(2(\tau))+\cos(2(\tau)))}{2\mu^2\omega^2+2}}} d\tau \quad [53]$$

$$\beta_2(\nu_1, \nu_2) = \frac{1}{\pi} \int_{-\pi}^{\pi} \frac{(\nu_1 + \nu_2 \sin(\tau)) \sin(\tau)}{\sqrt{\nu_1^2 + \frac{\nu_2^2}{2} - \frac{4\nu_1\nu_2(\mu\omega \cos(\tau)-2\sin(\tau))}{\mu^2\omega^2+4} - \frac{\nu_2^2(\mu\omega \sin(2(\tau))+\cos(2(\tau)))}{2\mu^2\omega^2+2}}} d\tau \quad [54]$$

$$\beta_3(\nu_1, \nu_2) = \frac{1}{\pi} \int_{-\pi}^{\pi} \frac{(\nu_1 + \nu_2 \sin(\tau)) \cos(\tau)}{\sqrt{\nu_1^2 + \frac{\nu_2^2}{2} - \frac{4\nu_1\nu_2(\mu\omega \cos(\tau)-2\sin(\tau))}{\mu^2\omega^2+4} - \frac{\nu_2^2(\mu\omega \sin(2(\tau))+\cos(2(\tau)))}{2\mu^2\omega^2+2}}} d\tau \quad [55]$$

In the case when  $\mu\omega = \mathcal{O}(\varepsilon)$ , a singular perturbation calculation leads to the quasi steady approximation:

$$\eta(\sigma) \approx \text{sign}(\nu_1 + \nu_2 \sin(\sigma + \phi + \phi_0)) + \mathcal{O}(\varepsilon) \quad [56]$$

for which the coefficients  $\beta_1(\nu_1, \nu_2), \beta_2(\nu_1, \nu_2), \beta_3(\nu_1, \nu_2)$  become:

$$\beta_1(\nu_1, \nu_2) = \begin{cases} \text{sign}(\nu_1) & |\nu_1| \geq |\nu_2| \\ \frac{2}{\pi} \text{sign}(\nu_1) \arcsin\left(\left|\frac{\nu_1}{\nu_2}\right|\right) & |\nu_1| < |\nu_2| \end{cases}, \quad \beta_2(\nu_1, \nu_2) = \begin{cases} 0 & |\nu_1| \geq |\nu_2| \\ \frac{4}{\pi} \text{sign}(\nu_2) \sqrt{1 - \left|\frac{\nu_1}{\nu_2}\right|^2} & |\nu_1| < |\nu_2| \end{cases}, \quad \beta_3(\nu_1, \nu_2) = 0$$

One can see that the gains  $\beta_1, \beta_2$  satisfy the relation:

$$\beta_1(\nu_1, \nu_2)^2 + \beta_2(\nu_1, \nu_2)^2 = \begin{cases} 1 & |\nu_1| \geq |\nu_2| \\ \frac{4}{\pi^2} \arcsin\left(\left|\frac{\nu_1}{\nu_2}\right|\right)^2 + \frac{16}{\pi^2} \left(1 - \left|\frac{\nu_1}{\nu_2}\right|^2\right) & |\nu_1| < |\nu_2| \end{cases} \quad [57]$$

from which it is easy to see that  $\beta_1(\nu_1, \nu_2), \beta_2(\nu_1, \nu_2)$  satisfy the inequality:

$$1 \leq \beta_1(\nu_1, \nu_2)^2 + \beta_2(\nu_1, \nu_2)^2 \leq \frac{16}{\pi^2} \approx 1.62 \quad [58]$$

as long as  $\nu_1^2 + \nu_2^2 \neq 0$ . Let us define the gains  $\rho_1$  and  $\rho_2$  by:

$$\rho_1 = \left| \frac{\beta_1(\nu_1, \nu_2)}{v\nu_1} \right|, \quad \rho_2 = \left| \frac{\beta_2(\nu_1, \nu_2)}{v\nu_2} \right| \quad [59]$$

and observe that under this definition, the gains  $\beta_1(\nu_1, \nu_2)$  and  $\beta_2(\nu_1, \nu_2)$  can now be written as:

$$\beta_1(\nu_1, \nu_2) = \rho_1(\nu_1, \nu_2) \nu_1 v, \quad \beta_2(\nu_1, \nu_2) = \rho_2(\nu_1, \nu_2) \nu_2 v \quad [60]$$

which implies that the quasi steady approximation of  $\eta(\tau)$  is now:

$$\eta(\tau) \approx v\rho_1(\nu_1, \nu_2)\nu_1 + v\rho_2(\nu_1, \nu_2)\nu_2 \sin(\tau) \quad \implies \quad \eta(t) \approx v\rho_1\nu_1 + v\rho_2\nu_2 \sin(\omega t + \phi + \phi_0) \quad [61]$$

Recalling equation [38] and [48] and the definition of  $\tau$ , one can see that in the original time variable  $t$ , the signal  $\eta(t)$  can be approximated in the quasi steady sense by:

$$\eta(t) \approx (\rho_1 \bar{\mathbf{V}} + \rho_2 \delta(\omega t + \phi))^\top \bar{\mathbf{R}}(t)^\top \frac{\nabla c(\bar{\mathbf{p}}(t))}{\|\nabla c(\bar{\mathbf{p}}(t))\|} \quad [62]$$

Using this expression for  $\eta(t)$ , the kinematics become:

$$\dot{\bar{\mathbf{p}}}(t) = \bar{\mathbf{R}}(t) \mathbf{V}_\eta(\omega t) \eta(t) \varepsilon + \bar{\mathbf{R}}(t) \bar{\mathbf{V}} \quad [63]$$

$$\dot{\bar{\mathbf{R}}}(t) = \bar{\mathbf{R}}(t) \hat{\boldsymbol{\Omega}}_\eta(\omega t) \eta(t) \quad [64]$$

where the feedback terms  $\mathbf{V}_\eta(\omega t) \eta(t)$  and  $\boldsymbol{\Omega}_\eta(\omega t) \eta(t)$  are given by:

$$\mathbf{V}_\eta(\omega t) \eta(t) = \mathbf{M}_1(\omega t) \bar{\mathbf{R}}(t)^\top \frac{\nabla c(\bar{\mathbf{p}}(t))}{\|\nabla c(\bar{\mathbf{p}}(t))\|} \quad [65]$$

$$\boldsymbol{\Omega}_\eta(\omega t) \eta(t) = \mathbf{M}_2(\omega t) \bar{\mathbf{R}}(t)^\top \frac{\nabla c(\bar{\mathbf{p}}(t))}{\|\nabla c(\bar{\mathbf{p}}(t))\|} \quad [66]$$

and the matrices  $\mathbf{M}_1$  and  $\mathbf{M}_2$  are given by:

$$\mathbf{M}_1(\omega t) = \left( \left( \omega_{\perp,1} \frac{\omega_{\parallel,0}}{\omega} - \omega_{\parallel,1} \frac{\omega_{\perp,0}}{\omega} \right) \mathbf{e}_1 - \left( \omega_{\parallel,1} \frac{\omega_{\parallel,0}}{\omega} + \omega_{\perp,1} \frac{\omega_{\perp,0}}{\omega} \right) \mathbf{e}_3(\omega t) \right) (\rho_1 \bar{\mathbf{V}} + \rho_2 \delta(\omega t + \phi))^\top \quad [67]$$

$$\mathbf{M}_2(\omega t) = \left( \left( \omega_{\parallel,1} \frac{\omega_{\parallel,0}}{\omega} + \omega_{\perp,1} \frac{\omega_{\perp,0}}{\omega} \right) \mathbf{e}_1 + \left( \omega_{\perp,1} \frac{\omega_{\parallel,0}}{\omega} - \omega_{\parallel,1} \frac{\omega_{\perp,0}}{\omega} \right) \mathbf{e}_3(\omega t) \right) (\rho_1 \bar{\mathbf{V}} + \rho_2 \delta(\omega t + \phi))^\top \quad [68]$$

Observe that

$$\delta(\omega t + \phi) = \frac{v\omega_{\perp,0}}{\omega} \mathbf{e}_2(\omega t + \phi) = \frac{v\omega_{\perp,0}}{\omega} \begin{pmatrix} \frac{\omega_{\perp,0}}{\omega} \sin(\omega t + \phi) \\ -\cos(\omega t + \phi) \\ -\frac{\omega_{\parallel,0}}{\omega} \sin(\omega t + \phi) \end{pmatrix} = \frac{v\omega_{\perp,0}}{\omega} \cos(\phi) \mathbf{e}_2(\omega t) + \frac{v\omega_{\perp,0}}{\omega} \sin(\phi) \mathbf{e}_3(\omega t) \quad [69]$$

Thus, we have:

$$\mathbf{M}_1(\omega t) = \left( \frac{\omega_{\perp,1}\omega_{\parallel,0} - \omega_{\parallel,1}\omega_{\perp,0}}{\omega} \right) \left( \frac{v\rho_1\omega_{\parallel,0}}{\omega} \mathbf{e}_1 \mathbf{e}_1^\top + \frac{v\rho_2\omega_{\perp,0}}{\omega} (\cos(\phi) \mathbf{e}_1 \mathbf{e}_2(\omega t)^\top + \sin(\phi) \mathbf{e}_1 \mathbf{e}_3(\omega t)^\top) \right) \quad [70]$$

$$- \left( \frac{\omega_{\parallel,1}\omega_{\parallel,0} + \omega_{\perp,1}\omega_{\perp,0}}{\omega} \right) \left( \frac{v\rho_1\omega_{\parallel,0}}{\omega} \mathbf{e}_3(\omega t) \mathbf{e}_1^\top + \frac{v\rho_2\omega_{\perp,0}}{\omega} (\cos(\phi) \mathbf{e}_3(\omega t) \mathbf{e}_2(\omega t)^\top + \sin(\phi) \mathbf{e}_3(\omega t) \mathbf{e}_3(\omega t)^\top) \right) \quad [71]$$

$$\mathbf{M}_2(\omega t) = \left( \frac{\omega_{\parallel,1}\omega_{\parallel,0} + \omega_{\perp,1}\omega_{\perp,0}}{\omega} \right) \left( \frac{v\rho_1\omega_{\parallel,0}}{\omega} \mathbf{e}_1 \mathbf{e}_1^\top + \frac{v\rho_2\omega_{\perp,0}}{\omega} (\cos(\phi) \mathbf{e}_1 \mathbf{e}_2(\omega t)^\top + \sin(\phi) \mathbf{e}_1 \mathbf{e}_3(\omega t)^\top) \right) \quad [72]$$

$$+ \left( \frac{\omega_{\perp,1}\omega_{\parallel,0} - \omega_{\parallel,1}\omega_{\perp,0}}{\omega} \right) \left( \frac{v\rho_1\omega_{\parallel,0}}{\omega} \mathbf{e}_3(\omega t) \mathbf{e}_1^\top + \frac{v\rho_2\omega_{\perp,0}}{\omega} (\cos(\phi) \mathbf{e}_3(\omega t) \mathbf{e}_2(\omega t)^\top + \sin(\phi) \mathbf{e}_3(\omega t) \mathbf{e}_3(\omega t)^\top) \right) \quad [73]$$

If we change to the time scale  $\sigma = \omega t$ , then the equations become:

$$\frac{d\bar{\mathbf{p}}}{d\sigma} = \varepsilon \bar{\mathbf{R}}(\sigma) \bar{\mathbf{V}} + \varepsilon^2 \bar{\mathbf{R}}(\sigma) \mathbf{V}_\eta(\sigma) \eta(\sigma) \quad [74]$$

$$\frac{d\bar{\mathbf{R}}}{d\sigma} = \varepsilon \bar{\mathbf{R}}(\sigma) \hat{\boldsymbol{\Omega}}_\eta(\sigma) \eta(\sigma) \quad [75]$$

which is on the canonical averaging form. Before we proceed, we compute some important time averages that will come up when we attempt to apply the averaging theorem:

$$\overline{\mathbf{e}_1 \mathbf{e}_2(\sigma)^\top} = 0, \quad \overline{\mathbf{e}_2(\sigma) \mathbf{e}_2(\sigma)^\top} = \frac{1}{2} (\mathbf{I} - \mathbf{e}_1 \mathbf{e}_1^\top), \quad \overline{\mathbf{e}_2(\sigma) \mathbf{e}_3(\sigma)^\top} = -\frac{1}{2} \hat{\mathbf{e}}_1 \quad [76]$$

$$\overline{\mathbf{e}_1 \mathbf{e}_3(\sigma)^\top} = 0, \quad \overline{\mathbf{e}_3(\sigma) \mathbf{e}_3(\sigma)^\top} = \frac{1}{2} (\mathbf{I} - \mathbf{e}_1 \mathbf{e}_1^\top), \quad \overline{\mathbf{e}_3(\sigma) \mathbf{e}_2(\sigma)^\top} = \frac{1}{2} \hat{\mathbf{e}}_1 \quad [77]$$

**2D Chemotaxis.** When the motion is confined to a plane, we will have that  $\omega_{\parallel,0} = \omega_{\parallel,1} = \rho_1 = 0$ , which greatly simplifies the expressions for the system. In particular, in the 2D case we will have:

$$\mathbf{M}_1(\sigma) = -v\rho_2\omega_{\perp,1}\text{sign}(\omega_{\perp,0}) (\cos(\phi)\mathbf{e}_3(\sigma)\mathbf{e}_2(\sigma)^\top + \sin(\phi)\mathbf{e}_3(\sigma)\mathbf{e}_3(\sigma)^\top) \quad [78]$$

$$\mathbf{M}_2(\sigma) = 0 \quad [79]$$

which leads to:

$$\frac{d\bar{\mathbf{p}}}{d\sigma} = \varepsilon^2 \bar{\mathbf{R}}(\sigma) \mathbf{M}_1(\sigma) \bar{\mathbf{R}}(\sigma)^\top \frac{\nabla c(\bar{\mathbf{p}}(\sigma))}{\|\nabla c(\bar{\mathbf{p}}(\sigma))\|} \quad [80]$$

$$\frac{d\bar{\mathbf{R}}}{d\sigma} = 0 \quad [81]$$

Moreover, the vector  $\mathbf{e}_1$  will be:

$$\mathbf{e}_1 = \begin{pmatrix} 0 \\ 0 \\ 1 \end{pmatrix} \quad [82]$$

By applying the averaging theorem to second order in  $\varepsilon$ , we obtain the system:

$$\frac{d\bar{\mathbf{p}}}{d\sigma} = \varepsilon^2 \bar{\mathbf{R}}(\sigma) \overline{\mathbf{M}_1(\sigma)} \bar{\mathbf{R}}(\sigma)^\top \frac{\nabla c(\bar{\mathbf{p}}(\sigma))}{\|\nabla c(\bar{\mathbf{p}}(\sigma))\|} \quad [83]$$

$$\frac{d\bar{\mathbf{R}}}{d\sigma} = 0 \quad [84]$$

where  $\overline{\mathbf{M}_1(\sigma)}$  is the time average of  $\mathbf{M}_1(\sigma)$ . Now, we compute:

$$\overline{\mathbf{M}_1(\sigma)} = -v\rho_2\omega_{\perp,1}\text{sign}(\omega_{\perp,0}) (\cos(\phi)\overline{\mathbf{e}_3(\sigma)\mathbf{e}_2(\sigma)^\top} + \sin(\phi)\overline{\mathbf{e}_3(\sigma)\mathbf{e}_3(\sigma)^\top}) = -\frac{v\rho_2\omega_{\perp,1}}{2} (\cos(\phi)\widehat{\mathbf{e}}_1 + \sin(\phi) (\mathbf{I} - \mathbf{e}_1\mathbf{e}_1^\top)) \quad [85]$$

Consequently, we obtain that the average local concentration evolves according to the differential equation:

$$\frac{d}{d\sigma} (c(\bar{\mathbf{p}}(\sigma))) = \nabla c(\bar{\mathbf{p}}(\sigma))^\top \frac{d\bar{\mathbf{p}}}{d\sigma} = \varepsilon^2 \nabla c(\bar{\mathbf{p}}(\sigma))^\top \bar{\mathbf{R}}(\sigma) \overline{\mathbf{M}_1(\sigma)} \bar{\mathbf{R}}(\sigma)^\top \frac{\nabla c(\bar{\mathbf{p}}(\sigma))}{\|\nabla c(\bar{\mathbf{p}}(\sigma))\|} \quad [86]$$

Since the motion is confined to a plane, we may assume, without loss of generality, that  $\mathbf{e}_1^\top \bar{\mathbf{R}}(\sigma)^\top \nabla c(\bar{\mathbf{p}}(\sigma)) = 0$ , which leads to:

$$\frac{d}{d\sigma} (c(\bar{\mathbf{p}}(\sigma))) = -\frac{v\rho_2\omega_{\perp,1}}{2} \text{sign}(\omega_{\perp,0}) \varepsilon^2 \nabla c(\bar{\mathbf{p}}(\sigma))^\top \bar{\mathbf{R}}(\sigma) (\cos(\phi)\widehat{\mathbf{e}}_1 + \sin(\phi)\mathbf{I}) \bar{\mathbf{R}}(\sigma)^\top \frac{\nabla c(\bar{\mathbf{p}}(\sigma))}{\|\nabla c(\bar{\mathbf{p}}(\sigma))\|} \quad [87]$$

$$= -\frac{v\rho_2\omega_{\perp,1}}{2} \text{sign}(\omega_{\perp,0}) \varepsilon^2 \sin(\phi) \|\nabla c(\bar{\mathbf{p}}(\sigma))\| \quad [88]$$

Going back to the time scale  $t = \varepsilon\sigma$ , we obtain the equation:

$$\frac{d}{dt} (c(\bar{\mathbf{p}}(t))) = -\frac{v\rho_2\omega_{\perp,1}}{2} \text{sign}(\omega_{\perp,0}) \varepsilon \sin(\phi) \|\nabla c(\bar{\mathbf{p}}(t))\| \quad [89]$$

Define the constant  $\gamma = \frac{v\rho_2\varepsilon}{2|\omega_{\perp,0}|}$ , and observe that the equation becomes:

$$\frac{d}{dt} (c(\bar{\mathbf{p}}(t))) = -\gamma \omega_{\perp,0} \omega_{\perp,1} \sin(\phi) \|\nabla c(\bar{\mathbf{p}}(t))\| \quad [90]$$

2 For successful 2D chemotaxis, it is required that  $\omega_{\perp,0}\omega_{\perp,1} \sin(\phi) < 0$ .

**3D Chemotaxis.** In the 3D case, the leading order behavior is the first order in  $\mathcal{O}(\varepsilon)$ . Hence, we compute only first order averaging:

$$\frac{d\bar{\mathbf{p}}}{d\sigma} = \varepsilon \bar{\mathbf{R}}(\sigma) \bar{\mathbf{V}} \quad [91]$$

$$\frac{d\bar{\mathbf{R}}}{d\sigma} = \varepsilon \bar{\mathbf{R}}(\sigma) \widehat{\bar{\mathbf{\Omega}}_\eta(\sigma)} \eta(\sigma) \quad [92]$$

where:

$$\widehat{\bar{\mathbf{\Omega}}_\eta(\sigma)} \eta(\sigma) = \overline{\mathbf{M}_2(\sigma)} \bar{\mathbf{R}}(\sigma)^\top \frac{\nabla c(\bar{\mathbf{p}}(\sigma))}{\|\nabla c(\bar{\mathbf{p}}(\sigma))\|} \quad [93]$$

We proceed with the averaging computation:

$$\overline{\mathbf{M}_2(\sigma)} = \frac{v\rho_1\omega_{\parallel,0}}{\omega} \left( \frac{\omega_{\parallel,1}\omega_{\parallel,0} + \omega_{\perp,1}\omega_{\perp,0}}{\omega} \right) \mathbf{e}_1 \mathbf{e}_1^\top + \frac{v\rho_2\omega_{\perp,0}}{2\omega} \left( \frac{\omega_{\perp,1}\omega_{\parallel,0} - \omega_{\parallel,1}\omega_{\perp,0}}{\omega} \right) (\cos(\phi)\widehat{\mathbf{e}}_1 + \sin(\phi)(\mathbf{I} - \mathbf{e}_1 \mathbf{e}_1^\top)) \quad [94]$$

If we define the unit vector  $\overline{\mathbf{q}}(\sigma) = \overline{\mathbf{R}}(\sigma)\mathbf{e}_1$ , we obtain that:

$$\frac{d\overline{\mathbf{q}}}{d\sigma} = \frac{d\overline{\mathbf{R}}}{d\sigma} \mathbf{e}_1 = \varepsilon \overline{\mathbf{R}}(\sigma) \widehat{\overline{\boldsymbol{\Omega}}_\eta(\sigma)\eta(\sigma)} \mathbf{e}_1 = \varepsilon \overline{\mathbf{R}}(\sigma) (\overline{\boldsymbol{\Omega}}_\eta(\sigma)\eta(\sigma) \times \mathbf{e}_1) = -\varepsilon \overline{\mathbf{R}}(\sigma) \widehat{\mathbf{e}}_1 \overline{\boldsymbol{\Omega}}_\eta(\sigma)\eta(\sigma) \quad [95]$$

$$= -\varepsilon \overline{\mathbf{R}}(\sigma) \widehat{\mathbf{e}}_1 \overline{\mathbf{M}_2(\sigma)} \overline{\mathbf{R}}(\sigma)^\top \frac{\nabla c(\overline{\mathbf{p}}(\sigma))}{\|\nabla c(\overline{\mathbf{p}}(\sigma))\|} \quad [96]$$

We compute:

$$\widehat{\mathbf{e}}_1 \overline{\mathbf{M}_2(\sigma)} = \frac{v\rho_2\omega_{\perp,0}}{2\omega} \left( \frac{\omega_{\perp,1}\omega_{\parallel,0} - \omega_{\parallel,1}\omega_{\perp,0}}{\omega} \right) (\cos(\phi)\widehat{\mathbf{e}}_1^2 + \sin(\phi)\widehat{\mathbf{e}}_1) \quad [97]$$

$$= \frac{v\rho_2\omega_{\perp,0}}{2\omega} \left( \frac{\omega_{\perp,1}\omega_{\parallel,0} - \omega_{\parallel,1}\omega_{\perp,0}}{\omega} \right) (\cos(\phi)(\mathbf{e}_1 \mathbf{e}_1^\top - \mathbf{I}) + \sin(\phi)\widehat{\mathbf{e}}_1) \quad [98]$$

Thus, we have:

$$\frac{d\overline{\mathbf{q}}}{d\sigma} = -\varepsilon \frac{v\rho_2\omega_{\perp,0}}{2\omega} \left( \frac{\omega_{\perp,1}\omega_{\parallel,0} - \omega_{\parallel,1}\omega_{\perp,0}}{\omega} \right) \overline{\mathbf{R}}(\sigma) (\cos(\phi)(\mathbf{e}_1 \mathbf{e}_1^\top - \mathbf{I}) + \sin(\phi)\widehat{\mathbf{e}}_1) \overline{\mathbf{R}}(\sigma)^\top \frac{\nabla c(\overline{\mathbf{p}}(\sigma))}{\|\nabla c(\overline{\mathbf{p}}(\sigma))\|} \quad [99]$$

$$= -\varepsilon \frac{v\rho_2\omega_{\perp,0}}{2\omega} \left( \frac{\omega_{\perp,1}\omega_{\parallel,0} - \omega_{\parallel,1}\omega_{\perp,0}}{\omega} \right) (\cos(\phi)(\overline{\mathbf{R}}(\sigma)\mathbf{e}_1 \mathbf{e}_1^\top \overline{\mathbf{R}}(\sigma)^\top - \mathbf{I}) + \sin(\phi)\overline{\mathbf{R}}(\sigma)\widehat{\mathbf{e}}_1 \overline{\mathbf{R}}(\sigma)^\top) \frac{\nabla c(\overline{\mathbf{p}}(\sigma))}{\|\nabla c(\overline{\mathbf{p}}(\sigma))\|} \quad [100]$$

$$= -\varepsilon \frac{v\rho_2\omega_{\perp,0}}{2\omega} \left( \frac{\omega_{\perp,1}\omega_{\parallel,0} - \omega_{\parallel,1}\omega_{\perp,0}}{\omega} \right) (\cos(\phi)(\overline{\mathbf{q}}(\sigma)\overline{\mathbf{q}}(\sigma)^\top - \mathbf{I}) + \sin(\phi)\widehat{\overline{\mathbf{q}}}(\sigma)) \frac{\nabla c(\overline{\mathbf{p}}(\sigma))}{\|\nabla c(\overline{\mathbf{p}}(\sigma))\|} \quad [101]$$

$$= -\varepsilon \frac{v\rho_2\omega_{\perp,0}}{2\omega} \left( \frac{\omega_{\parallel,1}\omega_{\perp,0} - \omega_{\perp,1}\omega_{\parallel,0}}{\omega} \right) \left( \cos(\phi)(\mathbf{I} - \overline{\mathbf{q}}(\sigma)\overline{\mathbf{q}}(\sigma)^\top) \frac{\nabla c(\overline{\mathbf{p}}(\sigma))}{\|\nabla c(\overline{\mathbf{p}}(\sigma))\|} - \sin(\phi)\overline{\mathbf{q}}(\sigma) \times \frac{\nabla c(\overline{\mathbf{p}}(\sigma))}{\|\nabla c(\overline{\mathbf{p}}(\sigma))\|} \right) \quad [102]$$

Recalling the definition of  $\overline{\mathbf{q}}$  and  $\overline{\mathbf{V}}$ , we see that:

$$\frac{d\overline{\mathbf{p}}}{dt} = \frac{v\omega_{\perp,0}}{\omega} \overline{\mathbf{q}} \quad \implies \quad \left\| \frac{d\overline{\mathbf{p}}}{dt} \right\|^2 = \frac{v^2\omega_{\perp,0}^2}{\omega^2} \quad \& \quad \frac{d^2\overline{\mathbf{p}}}{dt^2} = \frac{v\omega_{\perp,0}}{\omega} \frac{d\overline{\mathbf{q}}}{dt} \quad [103]$$

and also that:

$$\overline{\mathbf{q}}(t)\overline{\mathbf{q}}(t)^\top = \frac{\omega^2}{v^2\omega_{\perp,0}^2} \frac{d\overline{\mathbf{p}}}{dt} \frac{d\overline{\mathbf{p}}}{dt}^\top = \left\| \frac{d\overline{\mathbf{p}}}{dt} \right\|^{-2} \frac{d\overline{\mathbf{p}}}{dt} \frac{d\overline{\mathbf{p}}}{dt}^\top \quad [104]$$

Hence, by going back to the time scale  $t = \varepsilon\sigma$  we will have:

$$\frac{d^2\overline{\mathbf{p}}}{dt^2} = \gamma_1 \left( \mathbf{I} - \left\| \frac{d\overline{\mathbf{p}}}{dt} \right\|^{-2} \frac{d\overline{\mathbf{p}}}{dt} \frac{d\overline{\mathbf{p}}}{dt}^\top \right) \frac{\nabla c(\overline{\mathbf{p}}(t))}{\|\nabla c(\overline{\mathbf{p}}(t))\|} + \gamma_2 \frac{d\overline{\mathbf{p}}}{dt} \times \frac{\nabla c(\overline{\mathbf{p}}(t))}{\|\nabla c(\overline{\mathbf{p}}(t))\|} \quad [105]$$

where  $\gamma_1$  and  $\gamma_2$  are given by:

$$\gamma_1 = -\frac{\rho_2}{2} \frac{v^2\omega_{\perp,0}^2}{\omega^2} \left( \frac{\omega_{\parallel,1}\omega_{\perp,0} - \omega_{\perp,1}\omega_{\parallel,0}}{\omega} \right) \cos(\phi), \quad \gamma_2 = -\frac{\rho_2}{2} \frac{v^2\omega_{\perp,0}^2}{\omega^2} \left( \frac{\omega_{\parallel,1}\omega_{\perp,0} - \omega_{\perp,1}\omega_{\parallel,0}}{\omega} \right) \sin(\phi) \quad [106]$$

When the concentration field is linear:  $c(\mathbf{p}) = c_0 + \mathbf{c}_1^\top \mathbf{p}$ , a sufficient condition for successful positive chemotaxis is that  $\mathbf{c}_1^\top \frac{d\overline{\mathbf{p}}}{dt} > 0$ . If we show that  $\frac{d}{dt} (\mathbf{c}_1^\top \frac{d\overline{\mathbf{p}}}{dt}) > 0$  when  $\mathbf{c}_1^\top \frac{d\overline{\mathbf{p}}}{dt} < K$  for some positive nonzero constant  $K$ , then this means that  $\mathbf{c}_1^\top \frac{d\overline{\mathbf{p}}}{dt}$  is monotonically increasing which implies that eventually it will become positive. We proceed by the computation:

$$\frac{d}{dt} \left( \mathbf{c}_1^\top \frac{d\overline{\mathbf{p}}}{dt} \right) = \mathbf{c}_1^\top \frac{d^2\overline{\mathbf{p}}}{dt^2} = \gamma_1 \mathbf{c}_1^\top \left( \mathbf{I} - \left\| \frac{d\overline{\mathbf{p}}}{dt} \right\|^{-2} \frac{d\overline{\mathbf{p}}}{dt} \frac{d\overline{\mathbf{p}}}{dt}^\top \right) \frac{\mathbf{c}_1}{\|\mathbf{c}_1\|} = \gamma_1 \|\mathbf{c}_1\| \left( 1 - \|\mathbf{c}_1\|^{-2} \left\| \frac{d\overline{\mathbf{p}}}{dt} \right\|^{-2} \left( \mathbf{c}_1^\top \frac{d\overline{\mathbf{p}}}{dt} \right)^2 \right) \quad [107]$$

It is not hard to see that this quantity is positive as long as  $\mathbf{c}_1^\top \frac{d\overline{\mathbf{p}}}{dt} < \|\mathbf{c}_1\| \left\| \frac{d\overline{\mathbf{p}}}{dt} \right\|$  and  $\gamma_1 > 0$ . Thus, successful positive chemotaxis requires that

$$\gamma_1 > 0 \implies (\omega_{\parallel,1}\omega_{\perp,0} - \omega_{\perp,1}\omega_{\parallel,0}) \cos(\phi) < 0 \quad [108]$$
